# Supplementary material for: Snoopy: Sniffing Your Smartwatch Passwords via Deep Sequence Learning
Source: arXiv:1912.04836 source file (2019-12-11)
Supplement: Supplementary file 1 [file appendix.tex]

%!TEX root = ../snoopy.tex
\section*{Appendix}
\subsection*{Recurrent Neural Networks (RNNs) based Sequence Learning} 
\label{sub:basic_rnn}
In our context, the task of password inference is essentially learning a function between the password related motion data to the finite labels in the password database $P$. The motion data is inherently a time series, which captures the continuous posture changes of the smartwatch induced by user tapping or swiping. In addition, our problem is more challenging than standard sequence modelling since a) the input length can be variable, e.g. APLs can have different lengths, and b) the temporal correlations within data are strong, e.g. the likelihood of tapping on or swiping to a particular position depends very much on previous taps/swipes. Therefore, in this paper we use RNNs to model the motion data, which can take arbitrary length of input, and return the most likely password as output. In the following we explain how the standard RNN architecture solves this type of sequence learning problem. In the last two subsections we describe  how to extend the standard architecture to cope with our particular password inference problems. 

\noindent \textbf{Basic RNN Architecture:} 
Concretely, at each timestamp $\mathbf{k}$ a standard RNN keeps an internal hidden state $\mathbf{h}_k$ to describe the temporal dependencies, and given an input $\mathbf{x}_k$, the RNN updates its state by: 
\begin{equation}
\label{equ:rnn}
\begin{aligned}
   \mathbf{h}_k &= \mathcal{H}(\mathbf{W}_{xh}\mathbf{x}_k + \mathbf{W}_{hh}\mathbf{h}_{k-1} + \mathbf{b}_h)\\
   \mathbf{u}_k &= \mathbf{W}_{hu}\mathbf{h}_k + \mathbf{b}_u
\end{aligned}
\end{equation}
where $\mathbf{W}_{xh}$, $\mathbf{W}_{hh}$ are the weights of the current input $\mathbf{x}_k$ and previous state $\mathbf{h}_{k-1}$, and $\mathbf{b}_{h}$ is the bias vector. $\mathcal{H}$ is an element-wise non-linear activation function, e.g., sigmoid or hyperbolic tangent function. The network output $\mathbf{u}_k$ is evaluated as a linear combination of the updated  hidden state $\mathbf{h}_{k}$ and a bias vector $\mathbf{b}_{u}$. 

In practice, $\mathbf{u}_k$ may appear at multiple timestamp, or only exist at a single (in most cases the last) timestamp. The former type of network is able to map the input sequence to an output sequence, which is particularly useful in scenarios such as machine translation. The latter type generates a single output, for example a label based on the input sequence, and thus is often considered in applications such as text sentimental analysis. As discussed above, the password inference problem studied in this paper is to compute the most likely password (i.e. label) within the database $P$ given the sequence of motion data, which falls naturally into the latter category. Therefore in the following text, we only focus on those RNNs with a single output node, as shown in Fig.\ref{fig:archi_rnn} (Left).

\begin{figure*}[!t]
\centering
\includegraphics[width=0.5\columnwidth]{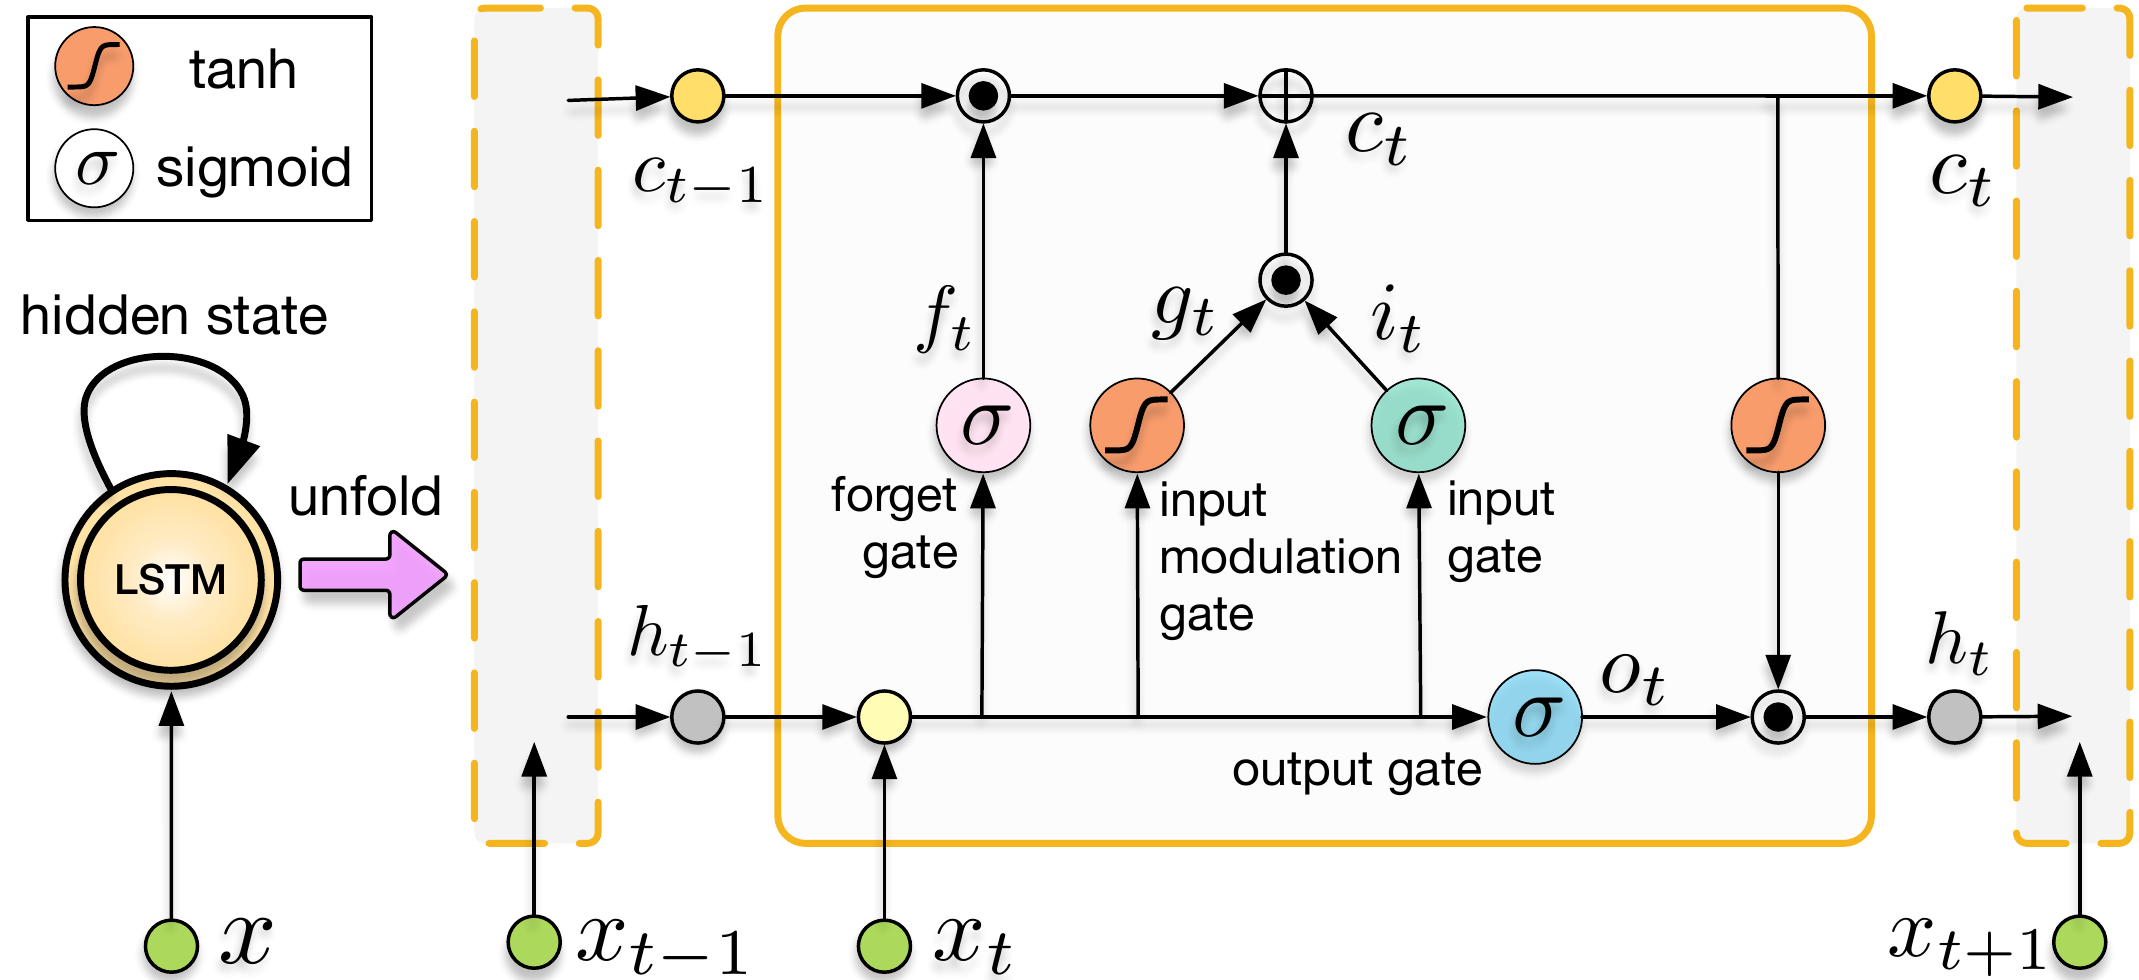}
\caption{Folded and unfolded LSTMs and the internal structures of its unit. $\odot$ and $\oplus$ denote element-wise product and addition of two vectors, respectively.}
\label{fig:rnn_cell}
\end{figure*}

\noindent \textbf{RNNs with LSTMs:} 
Although in theory the basic RNN is able to model sequences with arbitrary length, in practice it often suffers from the gradient vanishing and exploding problems~\cite{hochreiter2001gradient}. That is, it cannot capture the long-term dependencies well when the length of input sequences becomes large. Therefore for long input sequences, RNNs with Long Short Term Memory units (LSTMs)~\cite{hochreiter1997long}  are often considered. Essentially, LSTMs use self recurrent units (\emph{memory cells}) to explicitly determine which previous hidden states to ``remember'' or ``forget'', and thus provides a memory mechanism to capture dependencies spanning over many timesteps in the past. Fig.~\ref{fig:rnn_cell} shows an example of the LSTM units, in which the gates (forget/input/output) control the flow of information. Formally, the LSTM updates its own cell state $\mathbf{c}_k$ and the hidden state $\mathbf{h_k}$ as follows:

\begin{equation}
\label{equ:lstm}
\begin{aligned}
   \mathbf{i}_k &= \sigma(\mathbf{W}_{xi}\mathbf{x}_k + \mathbf{W}_{hi}\mathbf{h}_{k-1} + \mathbf{b}_i)\\
   \mathbf{g}_k &= \tanh(\mathbf{W}_{xg}\mathbf{x}_k + \mathbf{W}_{hg}\mathbf{h}_{k-1} + \mathbf{b}_g)\\
   \mathbf{f}_k &= \sigma(\mathbf{W}_{xf}\mathbf{x}_k + \mathbf{W}_{hf}\mathbf{h}_{k-1} + \mathbf{b}_f)\\
   \mathbf{c}_k &= \mathbf{f}_k\odot\mathbf{c}_{k-1} + \mathbf{i}_k\odot\mathbf{g}_k\\
   \mathbf{o}_k &= \sigma(\mathbf{W}_{xo}\mathbf{x}_k + \mathbf{W}_{ho}\mathbf{h}_{k-1} + \mathbf{b}_o)\\
   \mathbf{h}_k &= \mathbf{o}_k\odot\tanh(\mathbf{c}_k)
\end{aligned}
\end{equation}
where $\mathbf{i}_k$ and $\mathbf{g}_k$ are the input gates, i.e. govern which information in the previous hidden state $\mathbf{h_{k-1}}$ to remember, while $ \mathbf{f}_k$ is the forget gate that controls which part in $\mathbf{h_{k-1}}$ to forget, given the current input $\mathbf{x}_k$. The cell state $\mathbf{c}_k$ of this LSTM unit is then updated by combining information from those gates. $\mathbf{o}_k$ is the output gate, which is then fused with the current cell state $\mathbf{c}_k$ to update the hidden state $\mathbf{h_k}$. Note that $\sigma$ is the sigmoid function, $\texttt{tanh}$ is the hyperbolic tangent function, and $\odot$ is the element-wise product between vectors. 

\noindent \textbf{Cost Function and Optimisation: }
Given an input sequence $\mathbf{X} = (x_1, x_2, \cdots, x_T)$ with length of $T$  (in our case the 6 axis motion data), the above RNN essentially computes the likelihood of the labels $y \in \{1,2, \cdots, M\}$:
\begin{equation}
\label{equ:coditional_prob}
\begin{aligned}
    p(y|\mathbf{X}) &= p(y|x_1, x_2, \cdots, x_T) \\
                                &= softmax(\mathbf{W}_{hu}\mathbf{h}_T + \mathbf{b}_u)
\end{aligned}
\end{equation}
where we assume there is $M$ possible labels in total. If the true label $y$ is known for the input sequence $\mathbf{X}$, then training the network is equivalent to finding the optimal parameters (weights) $\theta$ where: 
\begin{equation}
   \theta^{*} =  \underset{\theta}{\argmax} \quad p(y|\mathbf{X};\theta)
\end{equation}
In practice, we typically use the cross entropy errors between the predicted and true labels as the cost function, which is defined as:
\begin{equation}
   \mathcal{L}(\mathbf{X}, y) = \sum_{j=1}^{M} \mathbf{1}\{y=j\}\log p(\widehat{y}_j)
\end{equation}
where $p(\widehat{y}_j)\in [0,1]$ is the probability of label $j$ predicted by the network, and $\mathbf{1} \{y=j\}$ is an indicator function which returns 1 if the true label $y$ is $j$. To optimize this cost function, there are various gradient-based techniques such as AdaGrad~\cite{duchi2011adaptive} and RMSProp~\cite{tieleman2012lecture}. In this paper we use Adam~\cite{kingma2014adam}, which combines the advantage of the two and is very efficient for training deep RNNs with LSTMs. 

\noindent \textbf{Regularization: }
Like other deep neuronal networks, the above RNNs with LSTMs can get overfit quickly. This is because by design the input of the network can have arbitrary length while the dimension of the output is fixed. Therefore through training, the RNNs tend to learn an input-dependent transition operator, which governs how to ``fold'' the variable length input sequences into the hidden states and ``squeeze'' them into fixed output vectors. However, as the training set won't cover sequences with all possible lengths, when applying the learned transition operator to an unseen test sequence, the dynamics of RNNs can be very sensitive to minor perturbations in the hidden states at different timestamps~\cite{krueger2016zoneout}. Therefore to make the RNNs practically useful, we need good regularization techniques to balance the fitness of training and generalization capability. In this paper, we consider a dropout technique inspired by~\cite{zaremba2014recurrent}, which randomly shuts down a subset of the network by disabling the corresponding feed-forward connections during training. Therefore, the dropout technique deliberately corrupts the information maintained by the memory units at some timestamps, but not all of them. In this way, we force the network to learn the general knowledge but not just specific features in the training data, and thus make it more robust in practice. 

% In Sec.~\ref{sec:evaluation} we will show that having an appropriate dropout strategy is key to successful password inference.

% Although the above RNNs with LSTMs have shown remarkable performance in many sequence learning problems, in our password inference problem such standard architecture doesn't work very well. One reason is that in our case, the input sequence of motion data can be very long. As shown in Fig.~\ref{fig:pwd_duration}, the duration of entering a password can be as long as $\sim$6 seconds ($\sim$1200 data points under the 200Hz sampling rate), which is very challenging even for LSTMs. Secondly, the characteristics of the motion data generated by PINs and APLs are very different (we will explain this in detail shortly), and thus it is inappropriate to simply use the same network architecture. To address this, Snoopy proposes two different network architectures based on standard deep RNNs, which are tailored for inferring PINs and APLs respectively.
